# Supplementary material for: Development of the Quantum Inspired SIBFA Many-Body Polarizable Force Field: Enabling Condensed Phase Molecular Dynamics Simulations
Source: arXiv:2201.00804 ancillary file (2022-05-16)
Supplement: Supplementary file 1 [file SI_SIBFA.pdf]

# Development of the Quantum Inspired SIBFA Many-Body Polarizable Force Field: I. Enabling Condensed Phase Molecular Dynamics Simulations


Sehr Naseem-Khan,[†,‡] Louis Lagardère,[*,†,¶] Christophe Narth,[†] G. Andrés Cisneros,[‡,§] Pengyu Ren,[‖] Nohad Gresh,[*,†] and Jean-Philip Piquemal[*,†,⊥,‖]

†*Sorbonne Université, LCT, UMR 7616 CNRS, 75005, Paris, France*

‡*Department of Chemistry, University of North Texas, Denton, TX 76201, USA*

¶*Sorbonne Université, IP2CT, FR 2622 CNRS,75005, Paris, France*

§*Present adress: Department of Physics, University of Texas at Dallas, TX 75080, USA*

‖*Department of Biomedical Engineering, The University of Texas at Austin, TX 78712, USA*

⊥*Institut Universitaire de France, 75005, Paris, France*

E-mail: louis.lagardere@sorbonne-universite.fr; nohad.gresh@lct.jussieu.fr; jean-philip.piquemal@sorbonne-universite.fr

# Supporting Information

## Contents


**1 Water dimers set used for the parametrization** **3**

**2 Energy Tables** **4**

**3 Auxiliary Figures and Tables** **7**

**4 Equations used to compute condensed phase properties** **9**

**5 SIBFA Parameters Files** **11**

**References** **21**

# 1 Water dimers set used for the parametrization

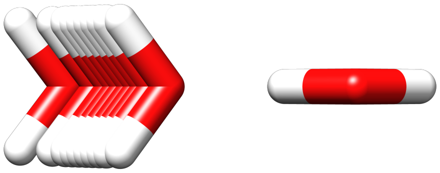

(a) Set-A

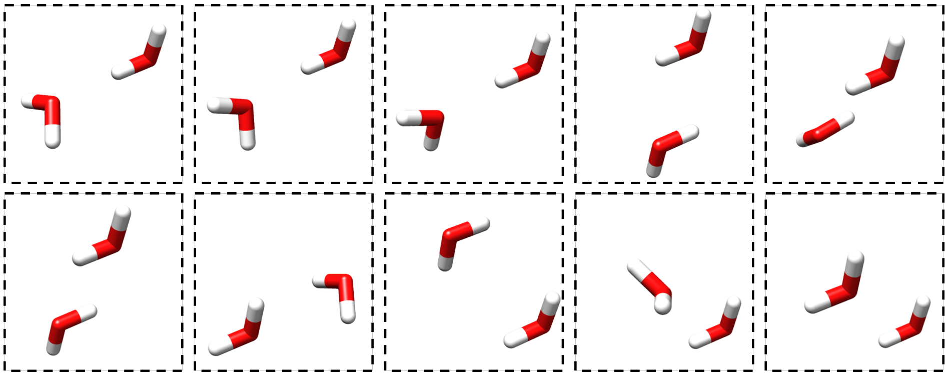

(b) Set-B

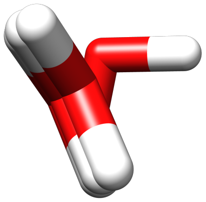

(c) Set-C

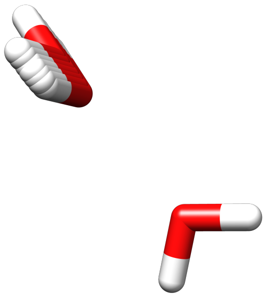

(d) Set-D

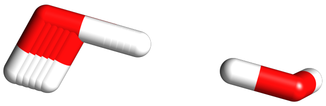

(e) Set-E

Figure S1: Representation of the water dimers used for the parametrization

a) Ten dimers from the radial scan of the linear water dimer monitoring the radial decay of both short- and long-range interactions between the oxygen of the H-bond acceptor and the interacting hydrogen of the H-bond donor. It also includes b) the ten dimers known as the Smith dimers,[1] representative of attractive and repulsive interactions between two water molecules. We have in addition included the following dimers: c) seven dimers in which the O of the second monomer approaches the O of the first along its external bisector; d) seven dimers in which the connecting O-O line is perpendicular to the plane of the first monomer.

In both c) and d), the two waters are perpendicular to one another, their H atoms being outward oriented, and the O-O distance vary from 2.4 to 3.0 Å; e) five dimers in which one H atom of the second molecule faces an H atom from the first, the corresponding OH bonds being colinear, and the H-H distance is varied from 1.5 to 2.0 Å. Clearly, c) and d) are considered so as to maximise the bond-bond, bond-lone pair, and lone pair-lone pair interactions, while e) is considered so as to maximise the H-H interactions as in the Ref.[2]

## 2 Energy Tables

**Table S1: Comparison of SIBFA21 and SAPT(DFT) energy components for the linear water dimer. The PBE0 functional and the aug-cc-pVTZ basis were used in SAPT(DFT) calculations.**

| d(Å) | 1.5 | 1.6 | 1.7 | 1.8 | 1.9 | 2.0 | 2.1 | 2.2 | 2.3 | 2.4 | 2.5 | 2.6 | 2.7 | 2.8 | 2.9 | 3.0 | RMSE |
|---|---|---|---|---|---|---|---|---|---|---|---|---|---|---|---|---|---|
| **Electrostatics** | | | | | | | | | | | | | | | | | |
| SAPT(DFT) | -20.63 | -16.37 | -13.10 | -10.58 | -8.64 | -7.13 | -5.96 | -5.04 | -4.31 | -3.72 | -3.25 | -2.86 | -2.53 | -2.26 | -2.03 | -1.83 | |
| SIBFA21 | -19.82 | -15.59 | -12.42 | -10.03 | -8.20 | -6.80 | -5.71 | -4.85 | -4.17 | -3.62 | -3.16 | -2.79 | -2.48 | -2.22 | -1.99 | -1.80 | 0.39 |
| **Exchange-Repulsion** | | | | | | | | | | | | | | | | | |
| SAPT(DFT) | 37.40 | 26.51 | 18.75 | 13.23 | 9.32 | 6.56 | 4.60 | 3.22 | 2.26 | 1.58 | 1.10 | 0.77 | 0.54 | 0.37 | 0.26 | 0.18 | |
| SIBFA21 | 37.53 | 25.47 | 17.35 | 11.85 | 8.11 | 5.57 | 3.83 | 2.64 | 1.82 | 1.26 | 0.87 | 0.60 | 0.42 | 0.29 | 0.20 | 0.14 | 0.74 |
| **Polarization** | | | | | | | | | | | | | | | | | |
| SAPT(DFT) | -2.62 | -2.10 | -1.69 | -1.35 | -1.08 | -0.87 | -0.69 | -0.56 | -0.45 | -0.36 | -0.30 | -0.24 | -0.20 | -0.16 | -0.14 | -0.11 | |
| SIBFA21 | -1.96 | -1.84 | -1.65 | -1.43 | -1.20 | -0.98 | -0.79 | -0.63 | -0.50 | -0.39 | -0.31 | -0.25 | -0.20 | -0.16 | -0.13 | -0.11 | 0.19 |
| **Charge Delocalization** | | | | | | | | | | | | | | | | | |
| SAPT(DFT) | -6.93 | -4.69 | -3.18 | -2.16 | -1.47 | -1.00 | -0.69 | -0.47 | -0.32 | -0.22 | -0.15 | -0.10 | -0.07 | -0.05 | -0.03 | -0.02 | |
| SIBFA21 | -3.91 | -2.91 | -2.17 | -1.62 | -1.21 | -0.90 | -0.67 | -0.50 | -0.37 | -0.28 | -0.21 | -0.15 | -0.11 | -0.09 | -0.06 | -0.05 | 0.93 |
| **Dispersion** | | | | | | | | | | | | | | | | | |
| SAPT(DFT) | -5.94 | -4.79 | -3.88 | -3.15 | -2.56 | -2.09 | -1.71 | -1.40 | -1.15 | -0.95 | -0.79 | -0.65 | -0.54 | -0.45 | -0.37 | -0.31 | |
| SIBFA21 | -5.57 | -4.40 | -3.52 | -2.85 | -2.33 | -1.91 | -1.57 | -1.31 | -1.09 | -0.91 | -0.76 | -0.64 | -0.54 | -0.46 | -0.39 | -0.33 | 0.20 |
| **Binding Energy** | | | | | | | | | | | | | | | | | |
| CCSD(T) | 0.96 | -1.85 | -3.48 | -4.35 | -4.72 | -4.78 | -4.64 | -4.40 | -4.10 | -3.77 | -3.45 | -3.14 | -2.85 | -2.58 | -2.34 | -2.12 | |
| SAPT(DFT) | 1.28 | -1.45 | -3.10 | -4.00 | -4.43 | -4.54 | -4.45 | -4.25 | -3.98 | -3.68 | -3.38 | -3.08 | -2.80 | -2.55 | -2.31 | -2.09 | 0.22 |
| SIBFA21 | 6.26 | 0.73 | -2.42 | -4.08 | -4.83 | -5.03 | -4.92 | -4.65 | -4.31 | -3.94 | -3.58 | -3.24 | -2.93 | -2.64 | -2.38 | -2.15 | 1.51 |

[a] $E_{\mathrm{cd}}^{(2)}(\mathrm{Reg}) + \delta_{\mathrm{HF}}^{(2)}$

**Table S2: Comparison of the binding energies computed with SIBFA21, AMOEBA+, AMOEBA14, and MB-UCB-MDQ to the *ab initio* reference computed at different level of theories : CCSD(T)/CBS for the trimer, tetramer, pentamer[3,4] and hexamers,[5] MP2/CBS for octamers[6] and 20 mers,[7] MP2/aug-cc-pV5Z (434,515,551) and MP2/aug-cc-pVQZ (443,4412) for endecamers[8] and CCSD(T)/aug-cc-pVTZ for 16 and 17 mers.[9] Values in kcal mol$^{-1}$.**

| Clusters | Ref | SIBFA21 | AMOEBA+ | AMOEBA14 | MB-UCB-MDQ |
|---|---|---|---|---|---|
| trimer | -15.74 | -16.20 | -16.07 | -15.38 | -16.07 |
| tretramer | -27.40 | -27.97 | -28.26 | -27.43 | -27.88 |
| pentamer | -35.93 | -35.91 | -36.41 | -35.78 | -37.23 |
| Hexamers | | | | | |
| prism | -45.92 | -47.48 | -46.03 | -45.18 | -43.11 |
| cage | -45.67 | -47.11 | -46.10 | -45.83 | -44.07 |
| bag | -44.30 | -45.05 | -44.65 | -44.52 | -44.06 |
| cyclic chair | -44.12 | -43.62 | -44.88 | -43.53 | -46.43 |
| book1 | -45.20 | -45.78 | -45.87 | -45.08 | -45.09 |
| book2 | -44.90 | -46.27 | -45.25 | -45.06 | -44.49 |
| cyclic boat1 | -43.13 | -42.80 | -43.54 | -42.99 | -45.01 |
| cyclic boat2 | -43.07 | -43.12 | -43.51 | -43.07 | -44.83 |
| Octamers | | | | | |
| $S_4$ | -72.70 | -76.67 | -73.56 | -72.22 | -72.53 |
| $D_{2d}$ | -72.70 | -76.79 | -73.74 | -72.24 | -72.54 |
| Endecamers | | | | | |
| 434 | -105.72 | -106.35 | -101.65 | -101.11 | -104.29 |
| 515 | -105.18 | -104.37 | -101.54 | -100.99 | -107.23 |
| 551 | -104.92 | -104.34 | -101.23 | -100.58 | -106.18 |
| 443 | -104.76 | -106.64 | -101.55 | -101.17 | -103.83 |
| 4412 | -103.97 | -104.40 | -100.94 | -100.33 | -105.24 |
| 16 mers | | | | | |
| boat-a | -170.80 | -168.15 | -162.50 | -160.45 | -167.92 |
| boat-b | -170.63 | -168.61 | -162.09 | -160.30 | -167.27 |
| antiboat | -170.54 | -167.57 | -161.77 | -160.30 | -166.45 |
| ABAB | -171.05 | -173.25 | -163.59 | -161.20 | -166.63 |
| AABB | -170.51 | -171.86 | -163.19 | -160.89 | -165.49 |
| 17 mers | | | | | |
| sphere | -182.54 | -179.10 | -172.24 | -171.53 | -180.68 |
| 5525 | -181.83 | -178.38 | -171.00 | -170.42 | -181.16 |
| 20 mers | | | | | |
| dodecahedron | -200.10 | -200.67 | -193.58 | -193.81 | -204.11 |
| fused cubes | -212.10 | -221.22 | -208.65 | -205.77 | -208.63 |
| face sharing prisms | -215.20 | -217.53 | -205.31 | -204.41 | -212.17 |
| edge sharing prisms | -218.10 | -219.28 | -208.53 | -207.06 | -213.58 |
| RMSE | | 2.54 | 5.45 | 6.33 | 2.48 |

**Table S3: Comparison of condensed phase properties computed with SIBFA21 to experiment[10] for the density ($\rho$), enthalpy of vaporization ($\Delta H_{\text{vap}}$), dielectric constant ($\epsilon_0$), isothermal compressibility ($\kappa_T$) and isobaric heat capacity ($C_p$). SIBFA21 values are obtained after using Bézier curves, except for $\epsilon_0$ where a linear square fit have been used.**

| | $\rho$ (g cm$^{-3}$) | | $\Delta H_{\text{vap}}$ (kcal mol$^{-1}$) | | $\epsilon_0$ | | $\kappa_T$ ($10^{-6}$ bar$^{-1}$ ) | | $C_p$ (cal mol$^{-1}$ K$^{-1}$) | |
|---|---|---|---|---|---|---|---|---|---|---|
| T(K) | Exp | SIBFA21 | Exp | SIBFA21 | Exp | SIBFA21 | Exp | SIBFA21 | Exp | SIBFA21 |
| 261 | 0.9975 | 1.0012 | 10.8893 | 12.4398 | 92.8980 | 90.0768 | 58.1160 | 58.6972 | 18.3800 | 29.8061 |
| 265 | 0.9986 | 1.0014 | 10.8431 | 12.3616 | 91.1860 | 88.7782 | 55.8510 | 55.4497 | 18.2800 | 29.1992 |
| 273 | 0.9998 | 1.0012 | 10.7714 | 12.2140 | 87.9030 | 86.5055 | 52.1760 | 50.368 | 18.1570 | 28.6168 |
| 277 | 1.0000 | 1.0007 | 10.7273 | 12.1442 | 86.3110 | 85.2069 | 50.6530 | 48.4985 | 18.1150 | 28.3933 |
| 281 | 0.9998 | 1.0001 | 10.6759 | 12.0802 | 84.7490 | 83.9082 | 49.2880 | 47.0156 | 18.0800 | 28.2317 |
| 285 | 0.9995 | 0.9994 | 10.6043 | 12.0186 | 83.2130 | 82.9342 | 48.0560 | 45.7526 | 18.0520 | 28.1341 |
| 289 | 0.9989 | 0.9985 | 10.6054 | 11.9545 | 81.7050 | 81.6356 | 46.9340 | 44.6253 | 18.0300 | 28.0782 |
| 293 | 0.9982 | 0.9974 | 10.5645 | 11.8813 | 80.2230 | 80.3369 | 45.8920 | 43.5976 | 18.0150 | 28.0251 |
| 298 | 0.9970 | 0.9961 | 10.5134 | 11.8083 | 78.4090 | 79.0383 | 45.2470 | 42.7953 | 18.0020 | 27.9570 |
| 309 | 0.9937 | 0.9923 | 10.4006 | 11.6174 | 74.5560 | 75.7917 | 44.3900 | 41.2262 | 17.9950 | 27.7266 |
| 321 | 0.9889 | 0.9880 | 10.2768 | 11.4242 | 70.5600 | 72.2204 | 44.1530 | 39.8894 | 18.0020 | 27.4907 |
| 333 | 0.9832 | 0.9828 | 10.1505 | 11.2128 | 66.7720 | 68.6491 | 44.4960 | 38.4754 | 18.0180 | 27.2731 |
| 345 | 0.9766 | 0.9767 | 10.0072 | 11.0013 | 63.1840 | 65.0778 | 45.3330 | 37.2338 | 18.0460 | 27.1049 |
| 353 | 0.9718 | 0.9725 | 9.9355 | 10.8692 | 60.8970 | 62.4805 | 46.1430 | 36.8477 | 18.0710 | 27.0346 |
| 369 | 0.9612 | 0.9638 | 9.7444 | 10.6274 | 56.5610 | 57.9352 | 48.3460 | 37.7725 | 18.1340 | 27.0637 |

# 3 Auxiliary Figures and Tables

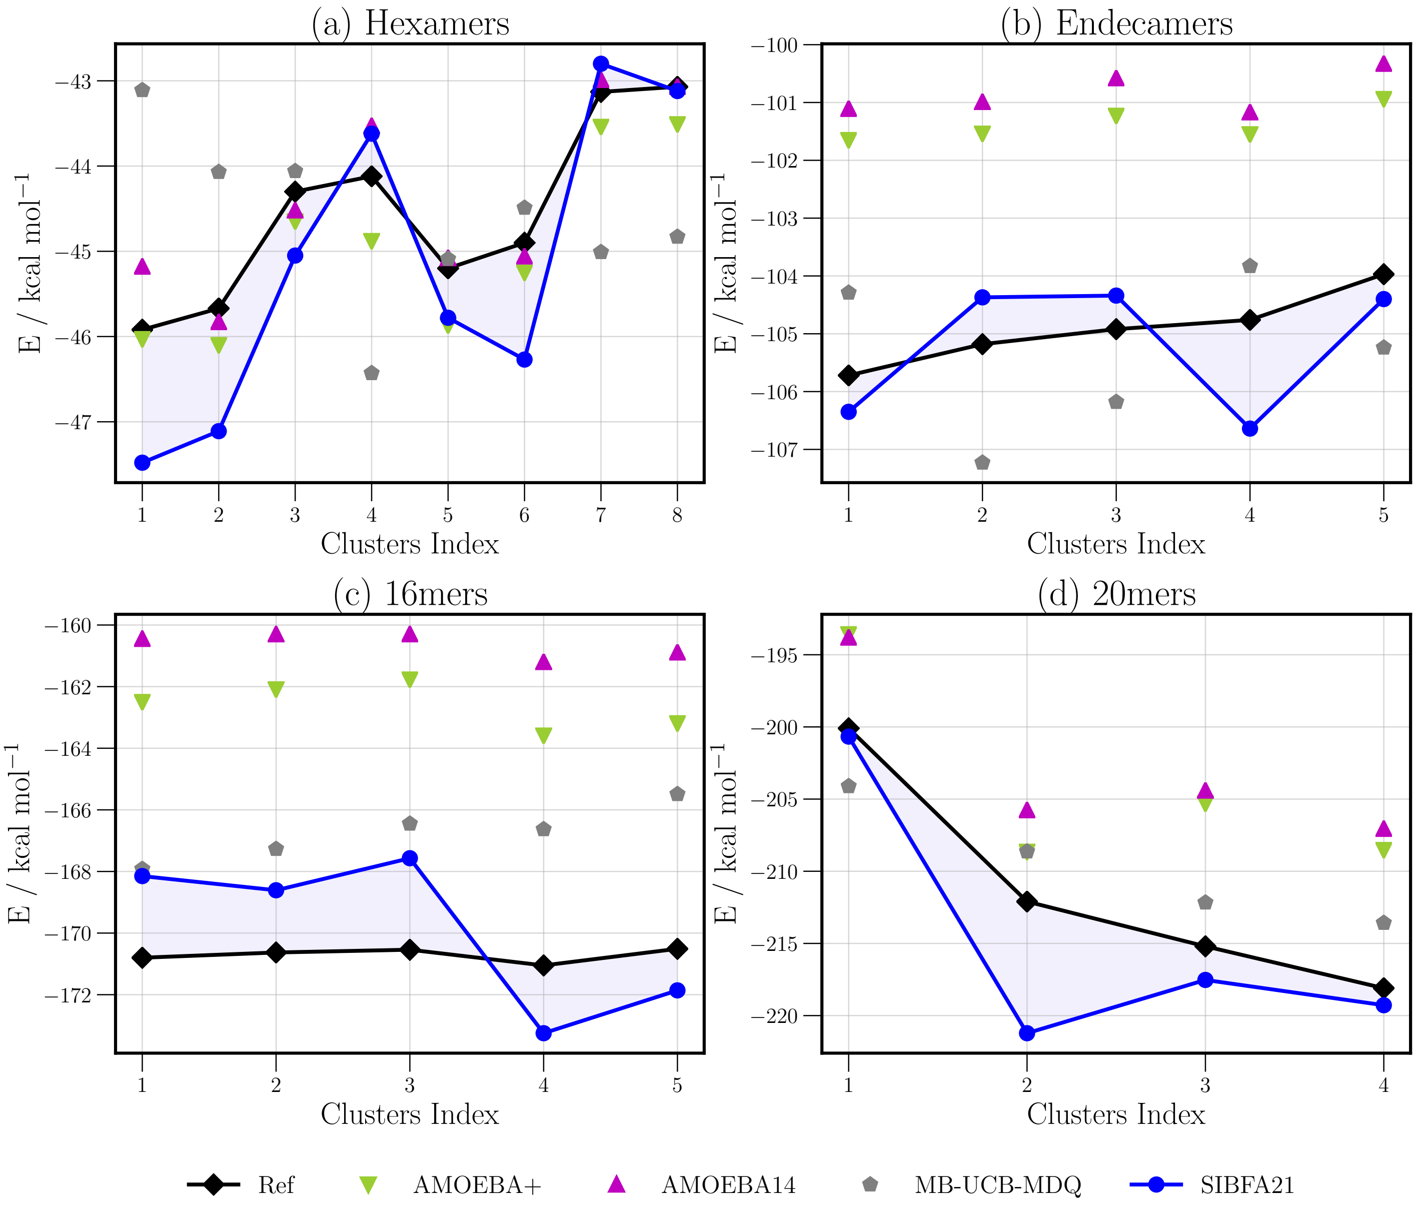


Figure S2: Comparison of the binding energies computed with SIBFA21, AMOEBA+, AMOEBA14, and MB-UCB-MDQ to the *ab initio* reference for different sizes of water clusters where the index corresponds to : (a) Hexamers : prim, cage, bag, cyclic-chair, book1, book2, cyclic-boat1, cyclic-boat2, (b) Endecamers : 434, 515, 551, 443, 4412, (c) boat-a, boat-b, anti-boat, ABAB, AABB and (d) 20mers : dodacahedron, fused cubes, face sharing prisms, edge sharing prisms.

**Table S4: Comparison of the binding energies computed with SIBFA21, AMOEBA+, AMOEBA14, and MB-UCB-MDQ to the CCSD(T)/CBS method for the Smith dimers.[1] The PBE0 functional and the aug-cc-pVTZ basis were used in SAPT(DFT) calculations. Values in kcal mol$^{-1}$.**

| Dimers | CCSD(T)/CBS[11] | CCSD(T)/aug-cc-pVTZ | SAPT(DFT) | SIBFA21 | AMOEBA+ | AMOEBA14 | MB-UCB-MDQ |
|---|---|---|---|---|---|---|---|
| 1 | -4.97 | -4.80 | -4.53 | -4.98 | -4.96 | -4.65 | -5.15 |
| 2 | -4.45 | -4.27 | -4.09 | -4.48 | -4.11 | -4.22 | -4.78 |
| 3 | -4.42 | -4.25 | -4.08 | -4.24 | -4.00 | -4.19 | -3.86 |
| 4 | -4.25 | -4.20 | -3.96 | -3.45 | -4.75 | -3.54 | -3.11 |
| 5 | -4.00 | -3.98 | -3.80 | -3.44 | -4.08 | -3.06 | -3.68 |
| 6 | -3.96 | -3.89 | -3.73 | -2.63 | -3.90 | -2.92 | -3.21 |
| 7 | -3.26 | -2.96 | -2.86 | -2.88 | -3.69 | -2.49 | -2.93 |
| 8 | -1.30 | -1.03 | -1.05 | -1.30 | -1.39 | -1.02 | -1.15 |
| 9 | -3.05 | -2.56 | -2.52 | -2.87 | -3.22 | -2.37 | -2.99 |
| 10 | -2.18 | -1.75 | -1.80 | -2.11 | -2.34 | -1.96 | -2.07 |
| RMSE | | 0.26 | 0.36 | 0.54 | 0.28 | 0.62 | 0.51 |

**Table S5: Condensed phase properties computed with SIBFA21, AMOEBA+, AMOEBA03, AMOEBA14, MB-UCB-MDQ and MB-POL at 298K: density ($\rho$), enthalpy of vaporization ($\Delta H_{\text{vap}}$), dielectric constant ($\epsilon_0$), isothermal compressibility ($\kappa_T$), isobaric heat capacity ($C_p$) and self-diffusion coefficient ($D$). SIBFA21 values are obtained after using Bézier curves, except for $\epsilon_0$ where a linear square fit have been used.**

| Properties | Exp | SIBFA21 | AMOEBA+ | AMOEBA03 | AMOEBA14 | MB-UCB-MDQ | MB-POL |
|---|---|---|---|---|---|---|---|
| $\rho$ (g cm$^{-3}$) | 0.997 | 0.996 | 0.998 | 1.0007 | 0.998 | 0.999 | 1.007 |
| $\Delta H_{\text{vap}}$ (kcal mol$^{-1}$) | 10.51 | 11.81 | 10.51 | 10.40 | 10.63 | 10.54 | 10.93 |
| $\epsilon_0$ | 78.41 | 79.03 | 80.40 | 90.40 | 79.40 | – | 68.40 |
| $C_p$ (cal mol$^{-1}$ K$^{-1}$) | 18.00 | 27.96 | – | 22.36 | 20.48 | – | 28.00 |
| $\kappa_T$ ($10^{-6}$ bar$^{-1}$ ) | 45.25 | 42.80 | 49.00 | 66.11 | 46.58 | – | 45.90 |
| $D$ ($10^{-5}$ cm$^2$ s$^{-1}$) | 2.29 | 1.47 | – | 2.00 | 1.99 | – | 2.34 |

# 4 Equations used to compute condensed phase properties

## 4.1 Enthalpy of vaporization

$$\Delta H_{\text{vap}} = U_{gas} - \frac{U_{liq}}{N} + RT \tag{1}$$

where $U_{gas} = 0.99$ kcal mol$^{-1}$ being the energy potential of one water molecule in the gas phase from the stochastic MD, $U_{gas}$ is the energy potential of the water from MD, $N$ is the number of water molecule in the box, $R$ is the gas constant and $T$, the temperature. Here, we assume the gas is ideal.

## 4.2 Dielectric Constant

$$\epsilon_0 = 1 + \frac{4\pi}{3k_B T\langle V\rangle}\Big(\langle M^2\rangle - \langle M\rangle\langle M\rangle\Big) \tag{2}$$

where $\langle M\rangle$ is the average of the dipole moment, $k_b$ is the Boltzmann constant, $\langle V\rangle$ the average volume of the water box and $T$ the temperature.

## 4.3 Isobaric Heat Capacity

$$C_p = \left(\frac{\delta U_{tot}}{\delta T}\right)_P \tag{3}$$

where $U_{tot}$ is the total energy from MD obtained and $T$ the temperature.

## 4.4 Isothermal Compressibility

$$\kappa_T = -\frac{1}{V}\left(\frac{\delta U_{tot}}{\delta T}\right)_{T,N} = \frac{1}{k_b T}\frac{\langle V^2\rangle - \langle V\rangle^2}{\langle V\rangle} \tag{4}$$

where $k_b$ is the Boltzmann constant, $\langle V\rangle$ the average volume of the water box and $T$ the temperature.

## 4.5 Self-Diffusion Coefficient

Einstein's relation:

$$D\pm = \lim_{t \to -\infty} \langle MSD(t)_{\pm} \rangle (6t)^{-1} \tag{5}$$

where $MSD(t)_{\pm}$ is the mean square displacement of the center of mass and $t$ the time.

**Self-Diffusion Coefficient - Size box correction** From ref.[12]

$$D_0 = D_{PBC} + 2.837297 \frac{k_b T}{6 \pi \eta L} \tag{6}$$

# 5 SIBFA Parameters Files

Below are the parameters files describing parameters for each contribution. For $E_{mtp}$, the two charge-charge penetration constants, the charge-dipole and the charge-quadrupole penetration constants, and the effective radii of O and H; for $E_{rep}$, the multiplicative constant and the exponent of the exponential; the internal coordinates of the lone pairs, the effective radii of O and H and the increment of effective radii along the direction of the lone pair; for $E_{pol}$, the isotropic scalar polarizabilites and Thole damping; for $E_{ct}$, the multiplicative constant and the exponent of the exponential; the effective radii of O and H; the increments of effective O radius along the direction of the lone pairs; for $E_{disp}$, the multiplicative constant; the effective radii of H and O; and the increments of effective O radius along the direction of the lone pairs.

## 5.1 SIBFA21 prm file

```
      ##############################
      ##                          ##
      ##  Force Field Definition  ##
      ##                          ##
      ##############################


forcefield              AMOEBA-WATER


bond-cubic              -2.55
bond-quartic            3.793125
angle-cubic             -0.014
angle-quartic           0.000056
```

```
angle-pentic            -0.0000007

angle-sextic            0.000000022

vdwtype                 BUFFERED-14-7

radiusrule              CUBIC-MEAN

radiustype              R-MIN

radiussize              DIAMETER

epsilonrule             HHG

dielectric              1.0

polarization            MUTUAL

polar-sor               0.75


      ##############################
      ##                          ##
      ##  Literature References   ##
      ##                          ##
      ##############################
```

P. Ren and J. W. Ponder, "A Polarizable Atomic Multipole Water Model for Molecular Mechanics Simulation", J. Phys. Chem. B, 107, 5933-5947 (2003)

Y. Kong, "Multipole Electrostatic Methods for Protein Modeling with Reaction Field Treatment", Ph.D. thesis, DBBS Program in Molecular Biophysics, Washington University, St. Louis, August, 1997 [available online from http://dasher.wustl.edu/ponder/]

```
alternative valence parameters to match symmetric and antisymmetric
bond stretches by David Semrouni, Ecole Polytechnique, Paris


      #############################
      ##                         ##
      ##  Atom Type Definitions  ##
      ##                         ##
      #############################


atom          1    1    O     "AMOEBA Water O"               8    15.995    2
atom          2    2    H     "AMOEBA Water H"               1     1.008    1


      ################################
      ##                            ##
      ##  Van der Waals Parameters  ##
      ##                            ##
      ################################


vdw           1               3.4050     0.1100
#vdw           1               0.0  0.0
vdw           2               2.6550     0.0135      0.910
```

```
      ##################################
      ##                              ##
      ##  Bond Stretching Parameters  ##
      ##                              ##
      ##################################


#bond          1    2           529.60     0.9572   !! original AMOEBA water
bond           1    2           556.85     0.9572


      ################################
      ##                            ##
      ##  Angle Bending Parameters  ##
      ##                            ##
      ################################


#angle         2    1    2       34.05     108.50   !! original AMOEBA water
angle          2    1    2       48.70     108.50


      ###############################
      ##                           ##
      ##  Urey-Bradley Parameters  ##
      ##                           ##
```

```
      ################################

#ureybrad     2    1    2      38.25     1.5537   !! original AMOEBA water
ureybrad      2    1    2      -7.60     1.5326

      ####################################
      ##                                ##
      ##  Atomic Multipole Parameters   ##
      ##                                ##
      ####################################

# ISA Multipoles computed with CamCASP
multipole     1   -2   -2              -0.83587
                                        0.00006   -0.00013   -0.15895
                                        0.37963
                                       -0.00039   -0.36802
                                        0.00012   -0.00003   -0.01161
multipole     2    1    2               0.41784
                                       -0.02428    0.00019   -0.01510
                                        0.00623
                                       -0.00008   -0.03192
                                        0.01317    0.00025    0.02569

      ########################################
```

```
      ##                                  ##
      ##  Dipole Polarizability Parameters  ##
      ##                                  ##
      ########################################


polarize      1           0.837      0.280       2
polarize      2           0.496      0.280       1


      ########################################
      ##                                  ##
      ##  Charge Penetration Parameters     ##
      ##                                  ##
      ########################################

sibfacp    1           4.0000     4.9000    4.7000
sibfacp    2           3.5000     2.9000    1.7000
#                      charge-charge charge-charge  charge-dipole charge-quad
sibfacporig            5.1749      4.2960    2.8433      2.1293
vdwcp      1           1.258
vdwcp      2           1.2803


      ################################################
      ##                                          ##
      ##  Charge Transfer Van der Waals Parameters  ##
```

```
##                                              ##
################################################

#                        donneur     accepteur
vdwct       1            1.4345d0   1.5077d0
vdwct       2            1.0d0      1.7513d0


#######################################################
##                                                   ##
## SIBFA Hybridation Cs and Cp parameters            ##
##                                                   ##
#######################################################

hybrid          1            0.5d0    0.866d0
hybrid          2            1.0d0    0.0d0


############################################
##                                        ##
##        ionisation potential            ##
##                                        ##
############################################

ah         1             12.78d0

############################################
```

```
      ##                                        ##
      ##        electronic affinity             ##
      ##                                        ##
      ############################################

ae        1             0.75d0
ae        2             0.75d0


      ############################################
      ##                                        ##
      ##        repulsion vdw parameter         ##
      ##                                        ##
      ############################################

vdwrep   1    1.4755d0
vdwrep   2    1.3469d0


      ############################################
      ##                                        ##
      ##        repulsion orbital parameter     ##
      ##                                        ##
      ############################################

gorb     1    1.36d0
gorb     2    1.0d0
```

```
#         cvrep11 cvrep12 41049.37629/192.7 41894.8999/192.7
coeffrep  213.022 217.4099
#         alpha alpha2
exprep     9.42905     15.918111

      ############################################
      ##                                        ##
      ##        dispersion     parameter        ##
      ##                                        ##
      ############################################

#vdwlpincrt(ect) need to be removed for lp vdw values
# 0.99-0.03576
vdwdisp   1    1.2594d0 0.90424 0.90424
vdwdisp   2    1.1767d0 1.0 1.0
#           C6disp C8disp C10disp scdp  facdispij discof colpa colp bdmp
coeffdisp   0.1166   0.0400 0.0030 -1.0 1.0  1.03  3.1961  6.0467     1.37
#          admp6 admp8 admp10 cxd   axd  cxdla    axdla  cxdlp  axdlp
expdisp    1.23  1.28 1.36 120.00 8.66398  120.006  7.455 120.00  8.88136
```

## 5.2 SIBFA21 key file

```
parameters         SIBFA2021_WATER.prm
#integrator respa
verbose
a-axis 18.643
ewald
ewald-cutoff 7
repulsion
rep-cutoff 7
dispersion
disp-cutoff 20
ctransferterm
ctransfer-cutoff 7 # first cutoff for lp(donnor)-acceptor interaction (first-circle)
ctnopot
mpolect-cutoff 7 # cutoff for potential on lp-acceptor (second circle)
#emtp
emtporig
archive
vdwterm none
randomseed 123
barostat montecarlo
polar-alg 1
#nlupdate 1
```

## 5.3 SIBFA21 LP file

```
4 Water Dimer
3 0 -0.083358311687338621 0.158270089447 -0.072676385841280597 1 2 1.9992300000000001 0.5 0.86599999999999999  -0.03576 0.000
3 0 -0.083358311687338621 -0.158270089447 -0.072676385841280597 1 2 1.9992300000000001 0.5 0.86599999999999999 -0.03576 0.000
6 0 -0.083358311687338621 0.158270089447 -0.072676385841280597 4 5 1.9992300000000001 0.5 0.86599999999999999  -0.03576 0.000
6 0 -0.083358311687338621 -0.158270089447 -0.072676385841280597 4 5 1.9992300000000001 0.5 0.86599999999999999 -0.03576 0.000
```

# References


(1) Smith, B. J.; Swanton, D. J.; Pople, J. A.; Schaefer, H. F.; Radom, L. Transition structures for the interchange of hydrogen atoms within the water dimer. *J. Chem. Phys.* **1990**, *92*, 1240–1247.

(2) Piquemal, J. P.; Chevreau, H.; Gresh, N. Toward a separate reproduction of the contributions to the Hartree-Fock and DFT intermolecular interaction energies by polarizable molecular mechanics with the SIBFA potential. *J. Chem. Theory Comput.* **2007**, *3*, 824–837.

(3) Dahlke, E. E.; Olson, R. M.; Leverentz, H. R.; Truhlar, D. G. Assessment of the Accuracy of Density Functionals for Prediction of Relative Energies and Geometries of Low-Lying Isomers of Water Hexamers. **2008**,

(4) Bates, D. M.; Tschumper, G. S. CCSD(T) complete basis set limit relative energies for low-lying water hexamer structures. *J. Phys. Chem. A* **2009**, *113*, 3555–3559.

(5) Wang, L.-P.; Head-Gordon, T.; Ponder, J. W.; Ren, P.; Chodera, J. D.; Eastman, P. K.; Martinez, T. J.; Pande, V. S. Systematic Improvement of a Classical Molecular Model of Water. *J. Phys. Chem. B* **2013**, *117*, 9956–9972.

(6) Xantheas, S. S.; Apra, E. The binding energies of the D-2d and S-4 water octamer isomers: High-level electronic structure and empirical potential results. *J. Chem. Phys.* **2004**, *120*, 823–828.

(7) Fanourgakis, G. S.; Aprà, E.; Xantheas, S. S. High-level ab initio calculations for the four low-lying families of minima of (H2O)20. I. Estimates of MP2/CBS binding energies and comparison with empirical potentials. *J. Chem. Phys.* **2004**, *121*, 2655–2663.

(8) Bulusu, S.; Yoo, S.; Aprà, E.; Xantheas, S.; Zeng, X. C. Lowest-energy structures of water clusters (H 2O)n and (H 2O) 13. *J. Phys. Chem. A* **2006**, *110*, 11781–11784.

(9) Yoo, S.; Aprà, E.; Zeng, X. C.; Xantheas, S. S. High-level Ab initio electronic structure calculations of water clusters (H2O)16 and (H2O)17: A new global minimum for (H2O)16. *J. Phys. Chem. Lett.* **2010**, *1*, 3122–3127.

(10) Wagner, W.; Pruß, A. The IAPWS formulation 1995 for the thermodynamic properties of ordinary water substance for general and scientific use. *J. Phys. Chem. Ref. Data* **2002**, *31*, 387–535.

(11) van Duijneveldt-van de Rijdt, J.; Mooij, W.; van Duijneveldt, F. Testing the quality of some recent water–water potentials. *Phys. Chem. Chem. Phys.* **2003**, *5*, 1169–1180.

(12) Yeh, I. C.; Hummer, G. System-size dependence of diffusion coefficients and viscosities from molecular dynamics simulations with periodic boundary conditions. *J. Phys. Chem. B* **2004**, *108*, 15873–15879.
